# Supplementary material for: Planar Friction Modelling with LuGre Dynamics and Limit Surfaces
Source: arXiv:2308.01123 source file (2024-05-22)
Supplement: Supplementary file 1 [file appendix.tex]

\subsection{Skew ellipsoid approximation}\label{sec:skew_var}
\textcolor{blue}{The ellipsoid approximation of the limit surface defined in \eqref{eq:LS_vel} will always have zero tangential force under pure rotation around CoP. Although this is addressed in the reduced model by the pre-calculated and normalized limit surface, }

In this section, the estimation of the skew variables $s_x$ and $s_y$, based on $h(r_a, \mathbf{v})$ is presented. The skew variables play a crucial role in cases where the CoR coincides with the CoP, but the contact results in non-zero tangential friction forces, as depicted in Fig. \ref{fig:skew_variables} and \ref{fig:force_vel_line_grad}. The skew variables add a virtual tangential velocity based on $\omega$ to simulate the correct tangential forces. To determine the skew variables, we define a point $\mathbf{p}_s = \begin{bmatrix}
    \Delta x & \Delta y  \\
\end{bmatrix}^T$ so that when CoR is aligned with $\mathbf{p}_s$, all tangential friction forces are cancelled out, see Fig. \ref{fig:skew_variables}. Algorithm \ref{alg:skew_var} estimates the location of $\mathbf{p}_s$ by iteratively updating $\mathbf{v}$ to minimize the normalized tangential forces from $h(\mathcolor{blue}{r_{a}'}, \mathbf{v})$. Fig. \ref{fig:algorithm} illustrates the velocity update in algorithm \ref{alg:skew_var}, the corresponding velocity to the normalized forces is estimated with an ellipsoid approximation without the skew variables. The position of $\mathbf{p}_s$ can be pre-computed for a given contact surface and the skew variables can then be approximated by:
\begin{equation}
    s_x = -\frac{r_a}{\mathcolor{blue}{r_{a}'}} s_n \Delta y    \quad\mathrm{and}\quad 
    s_y = \frac{r_a}{\mathcolor{blue}{r_{a}'}} s_n \Delta x 
\end{equation}
where $s_n \in [0, 1]$ is a scaling factor that depends on the ratio between $\omega$ and the tangential velocity $\mathbf{v}_t$. $s_n$ is necessary as the virtual velocity is only accurate when CoR is close to CoP. $s_n$ is approximated by: 
\begin{equation}
    s_n = \frac{2}{\pi} \textrm{atan2}{\left(|\omega| r_a, \sqrt{\left(\frac{v_x \Delta x}{ || \mathbf{p}_s|| }\right)^2 + \left(\frac{v_y \Delta y}{ || \mathbf{p}_s|| }\right)^2} \right)}
\end{equation}
where $\mathbf{v}_t$ is scaled depending on each component's contribution to the virtual velocity. The scaling factor $s_n$ decreases as the CoR moves farther away from CoP.
  
\begin{figure}
    \centering
    \smallskip 
    \includegraphics[width=\columnwidth]{images/skew_variables2.pdf}
    \caption{The left-hand side illustrates that CoP and $\mathbf{p}_s$ do not coincide for a gradient line contact. The $\mathbf{p}_s$ for a 1D surface has an equal amount of pressure on either side, $p_1 = p_2$, and a rotation around $\mathbf{p}_s$, therefore, generates zero tangential force. CoP has zero moments due to the pressure, but a rotation around CoP can generate tangential forces. The right-hand side illustrates the concept for a 2D surface, where $\mathbf{p}_s$ is a rotation point with zero tangential forces.}
    \label{fig:skew_variables}
    \vspace*{-0.5cm}
\end{figure}

\begin{figure}
    \centering
    \smallskip 
    \includegraphics[width=0.8\columnwidth]{images/algorithm.pdf}
    \caption{Iterations in algorithm \ref{alg:skew_var}. The algorithm finds a velocity $\mathbf{v}$ where the tangential forces are zeros while the surface is rotating. The left-hand side illustrates a slice of the normalised limit surface for a gradient line contact, and the right-hand side illustrates the velocity update.}
    \label{fig:algorithm}
    \vspace*{-0.5cm}
\end{figure}

\begin{algorithm}
\footnotesize

\caption{Find CoR with zero tangential friction}\label{alg:skew_var}
\begin{algorithmic}
\State $\omega = 1$
\State $\begin{bmatrix}
    h_x & h_y & h_\tau
\end{bmatrix}^T = h(\mathcolor{blue}{r_{a}'}, \mathbf{v} = \begin{bmatrix}
    v_x = 0 & v_y = 0  & \omega\\
\end{bmatrix})$
\State $\hat{v}_{x0} = \hat{v}_{x} = \mathcolor{blue}{r_{a}'} \omega h_x $
\State $\hat{v}_{y0} = \hat{v}_{y} = \mathcolor{blue}{r_{a}'} \omega h_y$
\While{$\sqrt{h_x^2 + h_y^2} > \textit{tol}$}
\State $\begin{bmatrix}
    h_x & h_y & h_\tau
\end{bmatrix}^T = h(\mathcolor{blue}{r_{a}'}, \mathbf{v} = \begin{bmatrix}
   \hat{v}_{x} & \hat{v}_{y}  & \omega \\
\end{bmatrix})$
\If{$\hat{v}_{x0} \neq 0$}
    \State $\hat{v}_{x} \gets \hat{v}_{x} (\mathcolor{blue}{r_{a}'}\omega h_x+\hat{v}_{x0}) / \hat{v}_{x0}$
\EndIf
 \If{$\hat{v}_{y0} \neq 0$}
    \State $\hat{v}_{y} \gets \hat{v}_{y} (\mathcolor{blue}{r_{a}'}\omega h_y + \hat{v}_{y0}) / \hat{v}_{y0}$
\EndIf

 \EndWhile
\State $\Delta x = - \hat{v}_{y} /\omega $
\State $\Delta y = \hat{v}_{x} /\omega$
\State \textbf{return} $\mathbf{p}_s = \begin{bmatrix}
    \Delta x & \Delta y
\end{bmatrix}^T$
\end{algorithmic}

\end{algorithm}

\subsection{Proof of positive definiteness of $\mathbf{A}_\textrm{sym}$}\label{app:positive_definite}

Here it is shown that the symmetric of $\mathbf{A}$, namely $\mathbf{A}_\textrm{sym}=\frac{1}{2}(\mathbf{A}+\mathbf{A}^T)$, is a positive definite matrix by proving that its eigenvalues are positive positive. As one of the eigenvalues of $\mathbf{A}_\textrm{sym}$ is $1$ we will investigate the sign of the other two eigenvalues given by:
%\begin{equation}
%    \textrm{det} \left(\begin{bmatrix} 1-\lambda &  0 & \frac{s_x}{2} \\
%     0 &  1-\lambda  & \frac{s_y}{2} \\
%     \frac{s_x}{2} &  \frac{s_y}{2}  & r_a^2 - \lambda \\
%    \end{bmatrix} \right) = 0
%\end{equation}
%which results in:
%\begin{equation}
%    (1-\lambda)(\lambda^2 - (r_a^2 + 1)\lambda + r_a^2 - \frac{s_x^2}{4} - %\frac{s_y^2}{4}) = 0
%\end{equation}
%where one the eigenvalues is $\lambda = 1$. The other two can be solved with the %quadratic formula:
\begin{equation}
    \lambda = \frac{r^2+1}{2} \pm \sqrt{ \left(\frac{r^2+1}{2}\right)^2 - \left( r_a^2 - \frac{s_x^2}{4} - \frac{s_y^2}{4}\right)}
\end{equation}
For the eigenvalues to be positive the following condition must be true:
\begin{equation}\label{eq:r_a_s_x_inequality}
    4 r_a^2 > s_x^2 + s_y^2 
\end{equation}

Consider the worst case scenario of $s_x^2 + s_y^2 $ being as large as possible, that is $s_n = 1$, %we consider $s_x = \Delta x$ and $s_y = \Delta y$ when $s_n = 1$, 
and ignore $\frac{r_a}{r_{as}}$ as it is a linear scaling that affects both sides equally.
We also consider a contact surface that consists of two points each with an infinitesimal contact area. Let point $p_1$ be the origin with a normal force $f_n$, and point $p_2$ with normal force $\gamma f_n$ where $0<\gamma<\frac{1}{2}$. Without loss of generality,  we consider the two points on an one-dimensional contact line along the x-axis, that is $s_y=0$. The distance between the two points is $d$ and the location $x$ of the CoP is then:
\begin{equation}
    x = \frac{\gamma f_n d}{f_n(1+ \gamma)} = \frac{\gamma d}{1+\gamma}
\end{equation}
As the points $p_1$ and $p_2$ have an infinitesimal area each, the location $p_s = s_x$ of the CoR, where no tangential forces exist, is located infinitely close to $p_1$ as it has higher normal force. This implies $|s_x| < |\frac{\gamma d}{1+\gamma}|$. The corresponding radius $r_a$ of a circle contact when rotating around CoP can be calculated as follows:
\begin{equation}
    r_a (f_n (1+\gamma)) = f_n \frac{\gamma d}{1+\gamma} + f_n (d - \frac{\gamma d}{1+\gamma})
\end{equation}
and is given by:
\begin{equation}\label{eq:r_a_point}
    r_a = \frac{d}{1+\gamma}
\end{equation}
If we assume the worst ``one-dimensional'' case as $s_x = -\frac{\gamma d}{1+\gamma}$ and $s_y = 0$, then \eqref{eq:r_a_s_x_inequality} becomes  $2r_a > |s_x|$ that, in turn, yields:
\begin{equation}
    2 \frac{d}{1+\gamma} < \frac{\gamma d}{1+\gamma}
\end{equation}
which holds as $0 < \gamma < \frac{1}{2}$. Therefore, all eigenvalues are positive and $\mathbf{A}_{\textrm{sym}}$ is positive definite for all surfaces.
